# Supplementary material for: Control and Placement of Finite-Resolution Intelligent Surfaces in IoT Systems with Imperfect CSI
Source: arXiv:2212.08631 source file (2022-12-16)
Supplement: Supplementary file 1 [file Appendices_full_descrip.tex]

\section{Proof of Lemma~\ref{lemma:approx_prob}}

\label{appndx:proof_approx_prob}

\begin{proof}
For a given $\mathbf{\Theta}$, we have
\begin{align}
\label{eq:intersect_real_imag}
    &\Pr\Big(\Big|\textbf{g}^{[i]}\mathbf{\Theta}\textbf{h}^{[j]}+h_d^{[ji]}\Big|<\delta\Big|\mathbf{\Theta}\Big) \\ \nonumber
    & \quad \quad \quad \quad >\Pr\Big(\Big|Re\{\textbf{g}^{[i]}\mathbf{\Theta}\textbf{h}^{[j]}+h_d^{[ji]}\}\Big|<\frac{\delta}{\sqrt{2}}\Big|\mathbf{\Theta} \bigcap \Big|Im\{\textbf{g}^{[i]}\mathbf{\Theta}\textbf{h}^{[j]}+h_d^{[ji]}\}\Big|<\frac{\delta}{\sqrt{2}}\Big|\mathbf{\Theta}\Big).
\end{align}
We define $X\triangleq Re\{\textbf{g}^{[i]}\mathbf{\Theta}\textbf{h}^{[j]}+h_d^{[ji]}\}$ and $Y\triangleq Im\{\textbf{g}^{[i]}\mathbf{\Theta}\textbf{h}^{[j]}+h_d^{[ji]}\}$ to make the proof easier to understand. Then, to simplify \eqref{eq:intersect_real_imag}, we need to show that $|X|$ and $|Y|$ are independent. We note that the independence of $X$ and $Y$ leads to the independence of $|X|$ and $|Y|$ since applying any function to two independent variables does not change the independence property. Thus, we remove the absolute function from the rest of the proof. Furthermore, from Lemma~\ref{lemma:avg_variance}, we know that $X$ and $Y$ are two random variables, which are distributed based on zero-mean Gaussian distribution. Therefore, $X$ and $Y$ are independent if they are uncorrelated (i.e., $Cov(X,Y)=0$). Hence, to show $Cov(X,Y)$, we write
\begin{align}
    Cov(X,Y)=\mathbb{E}(XY)-\mathbb{E}(X)\mathbb{E}(Y)\overset{(a)}{=}\mathbb{E}(XY),
\end{align}
where $(a)$ holds because $X$ and $Y$ are zero-mean random variables. Then, we have
\begin{align}
\label{eq:e_xy_ini}
    \mathbb{E}(XY)=\mathbb{E}\Big\{Re\{\sum_{m=1}^Mg_{m}^{[i]}e^{j\theta_m}h_{m}^{[j]}+h_d^{[ji]}\}Im\{\sum_{m^{\prime}=1}^Mg_{m^{\prime}}^{[i]}e^{j\theta_{m^{\prime}}}h_{m^{\prime}}^{[j]}+h_d^{[ji]}\}\Big\}.
\end{align}
We use superscript $R$ and $I$ to denote the real and imaginary parts of the channels ($h_d^{[ji]},h_{m}^{[j]}$ and $g_{m}^{[i]}$) and rewrite \eqref{eq:e_xy_ini} as
\begin{align}
\label{eq:e_xy_first_zeros}
    \mathbb{E}(XY)&=\mathbb{E}\Big\{\Big[\sum_{m=1}^M(g_{m}^{[i]R}h_{m}^{[j]R}-g_{m}^{[i]I}h_{m}^{[j]I})cos \theta_m-(g_{m}^{[i]I}h_{m}^{[j]R}+g_{m}^{[i]R}h_{m}^{[j]I})sin \theta_m+h_d^{[ji]R}\Big] \\ \nonumber &\times \Big[\sum_{m^{\prime}=1}^M(g_{m^{\prime}}^{[i]R}h_{m^{\prime}}^{[j]R}-g_{m^{\prime}}^{[i]I}h_{m^{\prime}}^{[j]I})sin \theta_{m^{\prime}}+(g_{m^{\prime}}^{[i]I}h_{m^{\prime}}^{[j]R}+g_{m^{\prime}}^{[i]R}h_{m^{\prime}}^{[j]I})cos \theta_{m^{\prime}}+h_d^{[ji]I}\Big]\Big\}\\ \nonumber
    &\overset{(b)}{=}\underbrace{\mathbb{E}\{h_d^{[ji]R}h_d^{[ji]I}\}}_{=0}+\underbrace{\mathbb{E}\Big\{\Big[\sum_{m=1}^M(g_{m}^{[i]R}h_{m}^{[j]R}-g_{m}^{[i]I}h_{m}^{[j]I})cos \theta_m-(g_{m}^{[i]I}h_{m}^{[j]R}+g_{m}^{[i]R}h_{m}^{[j]I})sin \theta_m\Big]h_d^{[ji]I}\Big\}}_{=0}\\ \nonumber
    &+\underbrace{\mathbb{E}\Big\{\Big[\sum_{m^{\prime}=1}^M(g_{m^{\prime}}^{[i]R}h_{m^{\prime}}^{[j]R}-g_{m^{\prime}}^{[i]I}h_{m^{\prime}}^{[j]I})sin \theta_{m^{\prime}}+(g_{m^{\prime}}^{[i]I}h_{m^{\prime}}^{[j]R}+g_{m^{\prime}}^{[i]R}h_{m^{\prime}}^{[j]I})cos \theta_{m^{\prime}}\Big]h_d^{[ji]R}\Big\}}_{=0} \\ \nonumber
    &+\mathbb{E}\Big\{\Big[\sum_{m=1}^M(g_{m}^{[i]R}h_{m}^{[j]R}-g_{m}^{[i]I}h_{m}^{[j]I})cos \theta_m-(g_{m}^{[i]I}h_{m}^{[j]R}+g_{m}^{[i]R}h_{m}^{[j]I})sin \theta_m\Big] \\ \nonumber 
    &\times \Big[\sum_{m^{\prime}=1}^M(g_{m^{\prime}}^{[i]R}h_{m^{\prime}}^{[j]R}-g_{m^{\prime}}^{[i]I}h_{m^{\prime}}^{[j]I})sin \theta_{m^{\prime}}+(g_{m^{\prime}}^{[i]I}h_{m^{\prime}}^{[j]R}+g_{m^{\prime}}^{[i]R}h_{m^{\prime}}^{[j]I})cos \theta_{m^{\prime}}\Big]\Big\},
\end{align}
where $(b)$ is correct since $h_d^{[ji]R}$, $h_d^{[ji]I}$, $h_{m}^{[j]R},g_{m}^{[i]R}$, $h_{m}^{[j]I},g_{m}^{[i]I}$,$h_{m^{\prime}}^{[j]R},g_{m^{\prime}}^{[i]R}$, $h_{m^{\prime}}^{[j]I}$, and $g_{m^{\prime}}^{[i]I}$ are independent and $\mathbb{E}\{h_d^{[ji]R}\}=\mathbb{E}\{h_d^{[ji]I}\}=0$. Then, we derive $\mathbb{E}(XY)$ through two cases: (i) $m=m^{\prime}$; (ii) $m\neq m^{\prime}$. Below, we describe these cases.

$\bullet~\mathbf{m=m^{\prime}:}$ In this case, since $m=m^{\prime}$ and $\mathbb{E}(XY)$ should hold for any given value of $M$, we consider $M=1$ and simplify \eqref{eq:e_xy_first_zeros} as
\begin{align}
\label{eq:m_m_complete}
    &\mathbb{E}(XY)\\ \nonumber
    &=\mathbb{E}\Big\{\Big[(g_{m}^{[i]R}h_{m}^{[j]R}-g_{m}^{[i]I}h_{m}^{[j]I})cos \theta_m-(g_{m}^{[i]I}h_{m}^{[j]R}+g_{m}^{[i]R}h_{m}^{[j]I})sin \theta_m\Big] \\ \nonumber 
    &\times \Big[(g_{m}^{[i]R}h_{m}^{[j]R}-g_{m}^{[i]I}h_{m}^{[j]I})sin \theta_{m}+(g_{m}^{[i]I}h_{m}^{[j]R}+g_{m}^{[i]R}h_{m}^{[j]I})cos \theta_{m}\Big]\Big\}\\ \nonumber
    &= \mathbb{E}\Big\{\Big[(g_{m}^{[i]R}h_{m}^{[j]R}-g_{m}^{[i]I}h_{m}^{[j]I})(g_{m}^{[i]I}h_{m}^{[j]R}+g_{m}^{[i]R}h_{m}^{[j]I})(cos^2\theta_m-sin^2\theta_m)\Big] \\ \nonumber 
    &+\frac{1}{2}\mathbb{E}\Big\{\Big[(g_{m}^{[i]R}h_{m}^{[j]R}-g_{m}^{[i]I}h_{m}^{[j]I})^2-(g_{m}^{[i]I}h_{m}^{[j]R}+g_{m}^{[i]R}h_{m}^{[j]I})^2\Big]sin2\theta_m\Big\}\\ \nonumber
    &=\mathbb{E}\Big\{\Big[(h_{m}^{[j]R})^2-(h_{m}^{[j]I})^2\Big]g_{m}^{[i]R}g_{m}^{[i]I}cos2\theta_m+\Big[(g_{m}^{[i]R})^2-(g_{m}^{[i]I})^2\Big]h_{m}^{[j]R}h_{m}^{[j]I}cos2\theta_m\Big\}\\ \nonumber
    &+\frac{1}{2}\mathbb{E}\Big\{\Big[(g_{m}^{[i]R}h_{m}^{[j]R})^2+(g_{m}^{[i]I}h_{m}^{[j]I})^2-(g_{m}^{[i]I}h_{m}^{[j]R})^2-(g_{m}^{[i]R}h_{m}^{[j]I})^2-4g_{m}^{[i]R}g_{m}^{[i]I}h_{m}^{[j]R}h_{m}^{[j]I}\Big]sin2\theta_m\Big\}\\ \nonumber
    &\overset{(c)}{=}\mathbb{E}\Big\{\Big[(h_{m}^{[j]R})^2-(h_{m}^{[j]I})^2\Big]g_{m}^{[i]R}g_{m}^{[i]I}cos2\theta_m\Big\}+\mathbb{E}\Big\{\Big[(g_{m}^{[i]R})^2-(g_{m}^{[i]I})^2\Big]h_{m}^{[j]R}h_{m}^{[j]I}cos2\theta_m\Big\} \\ \nonumber
    &+\frac{1}{2}\Big(\mathbb{E}\Big\{(h_{m}^{[j]R})^2\big[(g_{m}^{[i]R})^2-(g_{m}^{[i]I})^2\big]\Big\}+\mathbb{E}\Big\{(h_{m}^{[j]I})^2\big[(g_{m}^{[i]I})^2-(g_{m}^{[i]R})^2\big]\Big\}\Big)sin2\theta_m \\ \nonumber
    &-2\mathbb{E}\Big\{g_{m}^{[i]R}g_{m}^{[i]I}h_{m}^{[j]R}h_{m}^{[j]I}\Big\}sin2\theta_m\\ \nonumber
    &\overset{(d)}{=}\mathbb{E}\Big\{\Big[(h_{m}^{[j]R})^2-(h_{m}^{[j]I})^2\Big]\Big\}\mathbb{E}\Big\{g_{m}^{[i]R}g_{m}^{[i]I}\Big\}cos2\theta_m+\mathbb{E}\Big\{\Big[(g_{m}^{[i]R})^2-(g_{m}^{[i]I})^2\Big]\Big\}\mathbb{E}\Big\{h_{m}^{[j]R}h_{m}^{[j]I}\Big\}cos2\theta_m \\ \nonumber
    &+\frac{1}{2}\Big(\mathbb{E}\Big\{(h_{m}^{[j]R})^2\Big\}\mathbb{E}\Big\{\big[(g_{m}^{[i]R})^2-(g_{m}^{[i]I})^2\big]\Big\}+\mathbb{E}\Big\{(h_{m}^{[j]I})^2\Big\}\mathbb{E}\Big\{\big[(g_{m}^{[i]I})^2-(g_{m}^{[i]R})^2\big]\Big\}\Big)sin2\theta_m\\ \nonumber
    &-2\mathbb{E}\Big\{h_{m}^{[j]R}h_{m}^{[j]I}\Big\}\mathbb{E}\Big\{g_{m}^{[i]R}g_{m}^{[i]I}\Big\}sin2\theta_m\\ \nonumber
    &\overset{(e)}{=}\underbrace{\mathbb{E}\Big\{\Big[(h_{m}^{[j]R})^2-(h_{m}^{[j]I})^2\Big]\Big\}}_{=0}\mathbb{E}\Big\{g_{m}^{[i]R}g_{m}^{[i]I}\Big\}cos2\theta_m+\underbrace{\mathbb{E}\Big\{\Big[(g_{m}^{[i]R})^2-(g_{m}^{[i]I})^2\Big]\Big\}}_{=0}\mathbb{E}\Big\{h_{m}^{[j]R}h_{m}^{[j]I}\Big\}cos2\theta_m \\ \nonumber
    &+\frac{1}{2}\Big(\mathbb{E}\Big\{(h_{m}^{[j]R})^2\Big\}\underbrace{\mathbb{E}\Big\{\big[(g_{m}^{[i]R})^2-(g_{m}^{[i]I})^2\big]\Big\}}_{=0}+\mathbb{E}\Big\{(h_{m}^{[j]I})^2\Big\}\underbrace{\mathbb{E}\Big\{\big[(g_{m}^{[i]I})^2-(g_{m}^{[i]R})^2\big]\Big\}}_{=0}\Big)sin2\theta_m \\ \nonumber
    &-2\mathbb{E}\Big\{h_{m}^{[j]R}h_{m}^{[j]I}\Big\}\underbrace{\mathbb{E}\Big\{g_{m}^{[i]R}g_{m}^{[i]I}\Big\}}_{=0}\Big)sin2\theta_m=0,
\end{align}
where $(c)$ happens since the expected value operator is linear, and $(d)$ and $(e)$ are true because (i) the real and imaginary parts of the channels are independent; (ii) $\mathbb{E}\Big\{(g_{m}^{[i]I})^2\Big\}=\mathbb{E}\Big\{(g_{m}^{[i]R})^2\Big\}$; (iii) $\mathbb{E}\Big\{g_{m}^{[i]R}\Big\}=\mathbb{E}\Big\{g_{m}^{[i]I}\Big\}=0$.

$\bullet~\mathbf{m\neq m^{\prime}}:$ In this case, we have
\begin{align}
\label{eq:four_terms}
    \mathbb{E}(XY)&=\mathbb{E}\Big\{\Big[\sum_{m=1}^M(g_{m}^{[i]R}h_{m}^{[j]R}-g_{m}^{[i]I}h_{m}^{[j]I})cos \theta_m-(g_{m}^{[i]I}h_{m}^{[j]R}+g_{m}^{[i]R}h_{m}^{[j]I})sin \theta_m\Big] \\ \nonumber 
    &\times \Big[\sum_{m^{\prime}=1}^M(g_{m^{\prime}}^{[i]R}h_{m^{\prime}}^{[j]R}-g_{m^{\prime}}^{[i]I}h_{m^{\prime}}^{[j]I})sin \theta_{m^{\prime}}+(g_{m^{\prime}}^{[i]I}h_{m^{\prime}}^{[j]R}+g_{m^{\prime}}^{[i]R}h_{m^{\prime}}^{[j]I})cos \theta_{m^{\prime}}\Big]\Big\}.
\end{align}

Then, we use the linear property of the expected value operator and break \eqref{eq:four_terms} into four terms as \eqref{eq:first_product}, \eqref{eq:second_product}, \eqref{eq:third_product}, and \eqref{eq:fourth_product}. Here are the details.
\begin{align}
\label{eq:first_product}
    &\mathbb{E}\Big\{\sum_{m=1}^M(g_{m}^{[i]R}h_{m}^{[j]R}-g_{m}^{[i]I}h_{m}^{[j]I})cos \theta_m\times \sum_{m^{\prime}=1}^M(g_{m^{\prime}}^{[i]R}h_{m^{\prime}}^{[j]R}-g_{m^{\prime}}^{[i]I}h_{m^{\prime}}^{[j]I})sin \theta_{m^{\prime}}\Big\} \\ \nonumber
    &\overset{(f)}{=}\mathbb{E}\Big\{\sum_{m=1}^M(g_{m}^{[i]R}h_{m}^{[j]R})cos \theta_m \sum_{m^{\prime}=1}^M(g_{m^{\prime}}^{[i]R}h_{m^{\prime}}^{[j]R})sin \theta_{m^{\prime}}\Big\}-\mathbb{E}\Big\{\sum_{m=1}^M(g_{m}^{[i]I}h_{m}^{[j]I})cos \theta_m \sum_{m^{\prime}=1}^M(g_{m^{\prime}}^{[i]R}h_{m^{\prime}}^{[j]R})sin \theta_{m^{\prime}}\Big\} \\ \nonumber
    &+\mathbb{E}\Big\{\sum_{m=1}^M(g_{m}^{[i]I}h_{m}^{[j]I})cos \theta_m \sum_{m^{\prime}=1}^M(g_{m^{\prime}}^{[i]I}h_{m^{\prime}}^{[j]I})sin \theta_{m^{\prime}}\Big\}-\mathbb{E}\Big\{\sum_{m=1}^M(g_{m}^{[i]R}h_{m}^{[j]R})cos \theta_m \sum_{m^{\prime}=1}^M(g_{m^{\prime}}^{[i]I}h_{m^{\prime}}^{[j]I})sin \theta_{m^{\prime}}\Big\} \\ \nonumber
    &\overset{(g)}{=}\mathbb{E}\Big\{\sum_{m=1}^M(g_{m}^{[i]R}h_{m}^{[j]R})cos \theta_m\Big\} \mathbb{E}\Big\{\sum_{m^{\prime}=1}^M(g_{m^{\prime}}^{[i]R}h_{m^{\prime}}^{[j]R})sin \theta_{m^{\prime}}\Big\} \\ \nonumber
    &-\mathbb{E}\Big\{\sum_{m=1}^M(g_{m}^{[i]I}h_{m}^{[j]I})cos \theta_m\Big\} \mathbb{E}\Big\{\sum_{m^{\prime}=1}^M(g_{m^{\prime}}^{[i]R}h_{m^{\prime}}^{[j]R})sin \theta_{m^{\prime}}\Big\} \\ \nonumber
    &+\mathbb{E}\Big\{\sum_{m=1}^M(g_{m}^{[i]I}h_{m}^{[j]I})cos \theta_m\Big\} \mathbb{E}\Big\{\sum_{m^{\prime}=1}^M(g_{m^{\prime}}^{[i]I}h_{m^{\prime}}^{[j]I})sin \theta_{m^{\prime}}\Big\} \\ \nonumber
    &-\mathbb{E}\Big\{\sum_{m=1}^M(g_{m}^{[i]R}h_{m}^{[j]R})cos \theta_m \Big\}\mathbb{E}\Big\{\sum_{m^{\prime}=1}^M(g_{m^{\prime}}^{[i]I}h_{m^{\prime}}^{[j]I})sin \theta_{m^{\prime}}\Big\}\\ \nonumber
    &\overset{(h)}{=}\sum_{m=1}^M\underbrace{\mathbb{E}\{g_{m}^{[i]R}\}}_{=0}\mathbb{E}\{h_{m}^{[j]R}cos \theta_m\} \sum_{m^{\prime}=1}^M\underbrace{\mathbb{E}\{g_{m^{\prime}}^{[i]R}\}}_{=0}\mathbb{E}\{h_{m^{\prime}}^{[j]R}sin \theta_{m^{\prime}}\}\\ \nonumber
    &-\sum_{m=1}^M\underbrace{\mathbb{E}\{g_{m}^{[i]I}\}}_{=0}\mathbb{E}\{h_{m}^{[j]I}cos \theta_m\} \sum_{m^{\prime}=1}^M\underbrace{\mathbb{E}\{g_{m^{\prime}}^{[i]R}\}}_{=0}\mathbb{E}\{h_{m^{\prime}}^{[j]R}sin \theta_{m^{\prime}}\} \\ \nonumber
    &+\sum_{m=1}^M\underbrace{\mathbb{E}\{g_{m}^{[i]I}\}}_{=0}\mathbb{E}\{h_{m}^{[j]I}cos \theta_m\} \sum_{m^{\prime}=1}^M\underbrace{\mathbb{E}\{g_{m^{\prime}}^{[i]I}\}}_{=0}\mathbb{E}\{h_{m^{\prime}}^{[j]I}sin \theta_{m^{\prime}}\}\\ \nonumber
    &-\sum_{m=1}^M\underbrace{\mathbb{E}\{g_{m}^{[i]R}\}}_{=0}\mathbb{E}\{h_{m}^{[j]R}cos \theta_m \}\sum_{m^{\prime}=1}^M\underbrace{\mathbb{E}\{g_{m^{\prime}}^{[i]I}\}}_{=0}\mathbb{E}\{h_{m^{\prime}}^{[j]I}sin \theta_{m^{\prime}}\}=0,
\end{align}
where $(f)$ follows the linear property of the expected value operator, and $(g)$ and $(h)$ are true because $h_d^{[ji]R}$, $h_d^{[ji]I}$, $h_{m}^{[j]R},g_{m}^{[i]R}$, $h_{m}^{[j]I},g_{m}^{[i]I}$,$h_{m^{\prime}}^{[j]R},g_{m^{\prime}}^{[i]R}$, $h_{m^{\prime}}^{[j]I}$, and $g_{m^{\prime}}^{[i]I}$ are independent.
Similar to \eqref{eq:first_product}, we can show that
\begin{align}
\label{eq:second_product}
    \mathbb{E}\Big\{\sum_{m=1}^M(g_{m}^{[i]R}h_{m}^{[j]R}-g_{m}^{[i]I}h_{m}^{[j]I})cos \theta_m\times \sum_{m^{\prime}=1}^M(g_{m^{\prime}}^{[i]I}h_{m^{\prime}}^{[j]R}-g_{m^{\prime}}^{[i]R}h_{m^{\prime}}^{[j]I})cos \theta_{m^{\prime}}\Big\}=0,
\end{align}
\begin{align}
\label{eq:third_product}
    \mathbb{E}\Big\{\sum_{m=1}^M(g_{m}^{[i]I}h_{m}^{[j]R}-g_{m}^{[i]R}h_{m}^{[j]I})sin \theta_m\times \sum_{m^{\prime}=1}^M(g_{m^{\prime}}^{[i]R}h_{m^{\prime}}^{[j]R}-g_{m^{\prime}}^{[i]I}h_{m^{\prime}}^{[j]I})sin \theta_{m^{\prime}}\Big\}=0,
\end{align}

\begin{align}
\label{eq:fourth_product}
    \mathbb{E}\Big\{\sum_{m=1}^M(g_{m}^{[i]I}h_{m}^{[j]R}-g_{m}^{[i]R}h_{m}^{[j]I})sin \theta_m\times \sum_{m^{\prime}=1}^M(g_{m^{\prime}}^{[i]I}h_{m^{\prime}}^{[j]R}-g_{m^{\prime}}^{[i]R}h_{m^{\prime}}^{[j]I})sin \theta_{m^{\prime}}\Big\}=0.
\end{align}

Therefore, using \eqref{eq:m_m_complete}, \eqref{eq:first_product}, \eqref{eq:second_product}, \eqref{eq:third_product}, and \eqref{eq:fourth_product} prove that $\mathbb{E}\{XY\}=0$, and this means that $X$ and $Y$ are independent.

As a result, for $j\in\{1,2,\ldots,K\}, j\neq i.$ we simplify \eqref{eq:intersect_real_imag} as 
\begin{align}
    &\Pr\Big(\Big|\textbf{g}^{[i]}\mathbf{\Theta}\textbf{h}^{[j]}+h_d^{[ji]}\Big|<\delta\Big|\mathbf{\Theta}\Big) \\ \nonumber
    &>\Pr\Big(\Big|Re\{\textbf{g}^{[i]}\mathbf{\Theta}\textbf{h}^{[j]}+h_d^{[ji]}\}\Big|<\frac{\delta}{\sqrt{2}}\Big|\mathbf{\Theta}\Big)\Pr\Big(\Big|Im\{\textbf{g}^{[i]}\mathbf{\Theta}\textbf{h}^{[j]}+h_d^{[ji]}\}\Big|<\frac{\delta}{\sqrt{2}}\Big|\mathbf{\Theta}\Big).
\end{align}
Since $Re\{\textbf{g}^{[i]}\mathbf{\Theta}\textbf{h}^{[j]}+h_d^{[ji]}\}$ is a zero-mean Gaussian random variable, we have
\begin{align}
    \Pr\Big(\Big|Re\{\textbf{g}^{[i]}\mathbf{\Theta}\textbf{h}^{[j]}+h_d^{[ji]}\}\Big|<\frac{\delta}{\sqrt{2}}\Big|\mathbf{\Theta}\Big)&=\int_{-\frac{\delta}{\sqrt{2}}}^{\frac{\delta}{\sqrt{2}}}\frac{1}{\sqrt{\pi \nu}}e^{\frac{-r^2}{\nu}}dr \\ \nonumber
    &\overset{(q)}{\approx}\int_{-\frac{\delta}{\sqrt{2}}}^{\frac{\delta}{\sqrt{2}}}\frac{1}{\sqrt{\pi \nu}}\Big[1-\frac{r^2}{\nu}+O (\frac{r^4}{\nu^2})\Big]dr\\ \nonumber
    &=\frac{1}{\sqrt{\pi \nu}} \Big[\sqrt{2}\delta-\frac{\delta^3}{3\sqrt{2}\nu}+O(\frac{r^5}{\nu^2}) \Big]\\ \nonumber
    &\overset{(\ell)}{\approx}(\frac{\sqrt{2}\delta}{\sqrt{\pi \nu}}), ~~ j\in\{1,2,\ldots,K\}, j\neq i,
\end{align}
where $(q)$ applies based on approximation from the Taylor expansion of $e^{\frac{-r^2}{\nu}}$, and $(\ell)$ holds since our goal is to have small $\delta$; therefore, we ignore the high orders of $\frac{r}{\nu}$.

Similarly, we obtain
\begin{align}
    \Pr\Big(\Big|Im\{\textbf{g}^{[i]}\mathbf{\Theta}\textbf{h}^{[j]}+h_d^{[ji]}\}\Big|<\frac{\delta}{\sqrt{2}}\Big|\mathbf{\Theta}\Big)\approx(\frac{\sqrt{2}\delta}{\sqrt{\pi \nu}}), ~~ j\in\{1,2,\ldots,K\}, j\neq i.
\end{align}

Hence, using (24) and (25) leads to
\begin{align}
    \Pr\Big(\Big|\textbf{g}^{[i]}\mathbf{\Theta}\textbf{h}^{[j]}+h_d^{[ji]}\Big|<\delta\Big|\mathbf{\Theta}\Big)&>(\frac{\sqrt{2}\delta}{\sqrt{\pi \nu}})^2, j\in\{1,2,\ldots,K\}, j\neq i,
\end{align}
which completes the proof.
\end{proof}
